# Supplementary material for: Multiple Object Tracking with Correlation Learning
Source: arXiv:2104.03541 source file (2021-04-08)
Supplement: Supplementary file 1 [file appendix.tex]

\appendix
\section{Architectural details}
\label{sec:appendix_architecture}
\mypar{Correlation Operator.} 
Table~\ref{tab:flops} illustrates the

\begin{table*}[t]
\center
\caption{A comparison of the correlation operator with non-local operator. When the size of the local region is $R$ , the FLOPs of non-local is about $H\times W/(R\times R)$ times more than the correlation operator.}
\begin{tabular}{l  x{150} x{150}}
\toprule
Operator & Correlation & Non-local \\
\shline
Input & $C_{in} \times L \times H \times W$ &  $C_{in} \times L \times H \times W$ \\
Output & $C_{in} \times L \times H \times W$ &  $C_{in} \times L \times H \times W$ \\
{\#}params & $C_{in} \times C_{inter} \times 2 + (2R+1)^2\times C_{in} $ & $C_{in} \times C_{inter} \times 4 $ \\
FLOPs & $ C_{inter} \times (2R+1)^2\times \times H \times W  $ & $C_{inter} \times H\times W\times H \times W  $ \\
\bottomrule
\end{tabular}
\label{tab:flops}
\end{table*}

\begin{figure}[t]
\includegraphics[width=0.5\textwidth]{img/cal.pdf}
\caption{The space and time complexities for Non-Local and local Correlation. }
\label{fig:cal}
\end{figure}

\begin{figure*}[t]
\includegraphics[width=0.99\textwidth]{img/arch.pdf}
\caption{Model diagrams. The numbers in the boxes represent the stride to the image. (a): Baseline DLA-34 used in CenterNet~\cite{centernet}. (b) Spatial Local Correlation DLA-34. We add 4 spatial local correlation module before each IDA module. }
\label{fig:arch}
\end{figure*}

\section{Architecture Parameters}

\section{Training Objective}

\section{More Results}
